# Supplementary material for: Solving, Tracking and Stopping Streaming Linear Inverse Problems
Source: arXiv:2201.05741 source file (2024-01-30)
Supplement: Supplementary file 1 [file appendix.tex]

%
%\section{Sub-Exponential Random Variables}\label{apdx:subex}
%
%Here, we prove two lemmas. First, we prove the converse of \cite[Proposition 2.9]{wainwright_2019} in order to verify the claim that the two characterizations of sub-Exponential random variables in \cref{def:SE} are equivalent. Second, we prove \cref{lemma:cons_se}.
%
%\begin{lemma}\label{lemma:tail-to-subexponential}
%    Given a centered random variable $x$ such that 
%    \begin{equation}\label{tailbound}
%        \max\{\mathbb{P}(x>\delta), \mathbb{P}(x<-\delta)\} \leq \left\{
%            \begin{array}{ll}
%                  \exp\left(\frac{-\delta^2}{2\sigma^2}\right) & 0 \leq \delta \leq \frac{\sigma^2}{\omega}\\
%                  \exp\left(\frac{-\delta}{2\omega}\right) & \delta \geq \frac{\sigma^2}{\omega}\\
%            \end{array} 
%            \right.,
%    \end{equation}
%    then $x \sim \text{SE}(\sigma,\omega)$.
%\end{lemma}
%\begin{proof}
%    From \cite[Theorem 2.13]{wainwright_2019} we have that a distribution 
%    is sub-Exponential if for all $\delta > 0$ there
%    exists constants $c_1,c_2$ such that $\mathbb{P}(|x| \geq \delta) \leq c_1 e^{-c_2\delta}$.
%    Since we know for $\delta \geq  \frac{\sigma^2}{\omega}$ we have 
%   \begin{equation}
%    \mathbb{P}(|x|>\delta) \leq 2\exp\left(\frac{-\delta}{2\omega}\right) 
%   \end{equation}
%    we can select $c_2 = \frac{1}{2 \omega}$. We can then use this value 
%    to selected $c_1$ such that for $0 \leq \delta \leq \frac{\sigma^2}{\omega}$
%    we have 
%    \begin{equation}
%        2\exp\left(\frac{-\delta^2}{2\sigma^2}\right) \leq  c_1 e^{\frac{-\delta}{2\omega}}.
%    \end{equation} 
%    Rearranging this inequality we have to choose $c_1$ such that for all $\delta > 0$
%    we have 
%    \begin{equation}\label{c1bound}
%        2\exp\left(\frac{-\delta^2}{2\sigma^2}+\frac{\delta}{2\omega}\right) < c_1.
%    \end{equation} 
%    To select $c_1$ we will choose it such that \cref{c1bound} holds for the 
%    $\delta$ that maximizes $2\exp\left(\frac{-\delta^2}{2\sigma^2}+\frac{\delta}{2\omega}\right)$. Since 
%    this is a smooth function, and we are searching for the maximum over a compact set, we know that this maximum exists.
%    Taking derivates of the exponents and setting them 
%    equal to zero gives us the maximizing $\delta = \frac{\sigma^2}{2\omega}$.
%    Plugging this in to \cref{c1bound} we now want to select $c_1$ such that 
%    \begin{equation}
%        2\exp\left(\frac{-\delta^2}{2\sigma^2}+\frac{\delta}{2\omega}\right) \leq 2 \exp \left( \frac{\sigma^2}{8\omega^2}\right) = c_1 .
%    \end{equation}
%    Doing this by construction we have that 
%    \begin{equation}
%        \mathbb{P}(|x|>\delta) \leq \left\{
%            \begin{array}{ll}
%                  2\exp\left(\frac{-\delta^2}{2\sigma^2}\right) & 0 \leq \delta \leq \frac{\sigma^2}{\omega}\\
%                  2\exp\left(\frac{-\delta}{2\omega}\right) & \delta \geq \frac{\sigma^2}{\omega}\\
%            \end{array} 
%            \right. \leq 2 \exp \left( \frac{\sigma^2}{8\omega^2}\right)\exp\left(\frac{-\delta}{2\omega}\right),
%    \end{equation}
%    which allows us to conclude that $x$ is sub-Exponential by \cite[Theorem 2.13]{wainwright_2019}.
%\end{proof}
%We next present the proof for sub-Exponential distributions being closed under constant scaling.
%\begin{lemma}[\cref{lemma:cons_se}]
%    If given a random variable $Y$  with $\ex[Y] = \mu$  such that $Y - \mu \sim \text{SE}(\sigma,\omega)$ then for constants $c_1,c_2$ where $c_2 \geq |c_1|$ it is the case that $c_1(Y -\mu) \sim \text{SE}(c_2\sigma,c_2 \omega)$.
%\end{lemma}
%\begin{proof}
%    Since $y$ is sub-Exponential we know that for all $|t| \leq 1/\omega$
%    \begin{equation}
%        \ex[\exp(t(Y-\mu))] \leq \exp\left(\frac{t^2\sigma^2}{2}\right).
%    \end{equation}
%    Therefore, if we define $v = tc_1$ we know that $|v| \leq 1/\omega$ 
%    \begin{equation}
%        \ex[\exp(v(Y-\mu))] \leq \exp\left(\frac{v^2\sigma^2}{2}\right).
%    \end{equation}
%    By expanding $v$ this gives us that for all $|t| \leq \frac{1}{\omega |c_2|} \leq \frac{1}{\omega |c_1|}$ we have that
%    \begin{equation}
%        \ex[\exp(tz)] \leq \exp\left(\frac{t^2(c_1\sigma)^2}{2}\right) \leq \exp\left(\frac{t^2(c_2\sigma)^2}{2}\right).
%    \end{equation}
%    This allows us to conclude that $z \sim \text{SE}(|c_2|\sigma,|c_2|\omega )$ 
%\end{proof}
%
%\section{Sub-Exponential Examples}\label{apdx:ex_subexp}
%We now move to showing that the examples presented in \cref{ex:rand_sub,ex:colloc} are sub-Exponential. We begin with the random subsets example.
%    \begin{proposition}[\cref{prop:submat}]
%    Let $A \in \mathbb{R}^{m \times n}$ and $b \in \mathbb{R}^m$ such that $\exists x^* \in \mathbb{R}^n$ where $Ax^* = b$.
%        Let $\mathcal{S}$ be a random subset of $\lbrace 1,\ldots,m \rbrace$ of size $p \leq m$. Let $S \in \mathbb{R}^{m \times p}$ be the matrix whose columns are the standard basis elements indexed by $\mathcal{S}$. Let $(\tilde A , \tilde b) = (S^\top A,S^\top b)$. Then, for any $x \in \mathbb{R}^n$ such that $Ax \neq b$,
%        \begin{equation} \label{row_subset:exp1}
%            \frac{\|\tilde{A} x - \tilde b\|^2_2 - \ex [\|\tilde A x - \tilde b\|^2_2]}{ \ex [\|\tilde A x - \tilde b\|^2_2]} \sim \text{SE}\left(\frac{m}{2p},{0}\right).
%        \end{equation}
%    \end{proposition}
%    \begin{proof}
%     By \cref{lemma:boundedSE}, all bounded random variables are sub-Exponential with $\omega = 0$. Thus, it is enough to show that the left-hand side of \cref{row_subset:exp} is bounded from below and above. To do this, let $a_i \in \mathbb{R}^n$ denote the $i^\text{th}$ row of $A$, and note that $\mathbb{P}(i \in \mathcal{S}) = p/m$. Therefore, $\ex [ \Vert \tilde A x - \tilde b \Vert_2^2] = \sum_{i = 1}^m \frac{p}{m} [a_i^\top (x - x^*)]^2.$
%        Using this calculation,
%    $
%            0 \leq \|\tilde A x - \tilde b\|^2_2 = \sum_{i \in \mathcal{S}} [a_i^\top (x - x^*)]^2 \leq \sum_{i = 1}^m [a_i^\top (x - x^*)]^2 = \frac{m}{p} \ex [\|\tilde A x - \tilde b \|^2_2].
%    $
%    
%    From this lower and upper bound on $\Vert \tilde A x - \tilde b \Vert_2^2$, we conclude that for any $x$ such that $Ax \neq b$,
%        \begin{equation}
%           -1 \leq  \left| \frac{\|\tilde{A}_k x - \tilde b_k\|^2_2 - \ex [\|\tilde A_k x - \tilde b_k\|^2_2]}{ \ex [\|\tilde A_k x - \tilde b_k\|^2_2]} \right| \leq \frac{m - p}{p}.
%        \end{equation}
%        The result follows.
%    \end{proof}
%We finish by presenting the proof that the collocation problem in \cref{ex:colloc} is sub-Exponential.
%\begin{proposition}[\cref{prop:colloc}]
%    Let $\lbrace t_1,\ldots,t_p \rbrace$ chosen independently and uniformly from both $(0,1)^3$ and $\partial [0,1]^3$. Let the entries of $\tilde A$ be defined according to \cref{eq:collocA} and those of $\tilde b$ be defined according to \cref{eq:collocb}. Then, if we let $D = \frac{9N}{\sigma_{\min}( \ex[ \tilde A^\top \tilde A])}$, where $\sigma_{\min}$ is the smallest non-zero singular value and $N$ is the number of columns in $\tilde A$, 
%    \begin{equation} \label{colloc:exp1}
%        \frac{\|\tilde{A}x - \tilde b\|^2 - \ex [\|\tilde A x - \tilde b\|^2]}{ \ex [\|\tilde A x - \tilde b\|^2]} \sim \text{SE}\left(\frac{D}{2},{0}\right). 
%    \end{equation}
%\end{proposition}
%\begin{proof}
%
%Let $x^* \in \mathbb{R}^n$ denote any vector such that $\mathbb{P}(\tilde A x^* = \tilde b) = 1$. For any $x \in \mathbb{R}^n$ such that $\mathbb{P}( \tilde A x = \tilde b) < 1$, we can decompose $x - x^*$ into $u \in \mathrm{row}( \ex [ \tilde A^\top \tilde A ])$ and $v \in \mathrm{null}( \ex [\tilde A^\top \tilde A ])$. By construction, $u \neq 0$. Moreover, $v \in \mathrm{null}( \ex[\tilde A^\top \tilde A])$ with probability one (otherwise we would have a contradiction with $v \in \mathrm{null}( \ex [\tilde A^\top \tilde A ])$).
%
%Therefore,
%\begin{equation}
%0 \leq \frac{ \Vert \tilde A x - \tilde b \Vert_2^2 }{ \ex[ \Vert \tilde A x - \tilde b \Vert_2^2   ] } = \frac{ \Vert \tilde A u \Vert_2^2 }{u^\top \ex [ \tilde A^\top \tilde A ] u} \leq \frac{ \Vert \tilde A \Vert_2^2 }{ \sigma_{\min}( \ex[ \tilde A^\top \tilde A] )},
%\end{equation}
%where $\sigma_{\min}$ denotes the smallest non-zero singular value of the given matrix. Using \cref{eq:collocA}, we can find the maximum possible value of $\tilde A$ on the unit cube is $3$ and thus using the equivalence between the infinity and two norms $\|\tilde A\|_2^2 \leq 9N$. So we can set $D = \frac{9N}{\sigma_{\min}( \ex[ \tilde A^\top \tilde A])}$.
%
%Hence,
%\begin{equation}
%-1 \leq \frac{ \Vert \tilde A x - \tilde b \Vert_2^2 }{ \ex[ \Vert \tilde A x - \tilde b \Vert_2^2   ] } - 1\leq D - 1.
%\end{equation}
%Applying \cref{lemma:boundedSE} gives the conclusion.
%\end{proof}
%
%
%\subsection{Consistency of $\tilde \rho_k$}\label{apdx:cons-of-rho}
%\begin{corollary}[\cref{cor:cons-of-rho}]
%    Suppose the setting of \cref{thm:convergence-of-moments} holds. Then, for any $\lambda \in \mathbb{N}$ and $\forall \delta > 0$, $\lim_{k \to \infty} \mathbb{P}( |\tilde \rho_k^\lambda - \rho_k^\lambda | > \delta) = 0$. That is, $\tilde \rho_k^\lambda$ is a consistent estimator of $\rho_k^\lambda$.
%    \end{corollary}
%    \begin{proof}
%        We begin by noting that
%        \begin{small}
%        \begin{align}
%            \lim_{k \to \infty} \mathbb{P}( |\tilde \rho_k^\lambda - \rho_k^\lambda | > \delta) &= \lim_{k \to \infty}\ex\left[\mathbb{I}_{|\tilde \rho_k^\lambda - \rho_k^\lambda | > \delta}\right]\\
%            &= \lim_{k \to \infty}\ex\left[\pr\left(|\tilde \rho_k^\lambda - \rho_k^\lambda | > \delta|\siga\right)\right]\label{eq:tower} \\
%            &\leq \lim_{k \to \infty}\ex \left[2e^{-\min\left\{\frac{\lambda \delta^2}{2\sigma^2\bound^2(1+\log(\lambda))},\frac{\delta}{2\omega\bound} \right\}}\right]\label{eq:bound_se}\\
%            &= \ex \left[\lim_{k \to \infty} 2e^{-\min\left\{\frac{\lambda \delta^2}{2\sigma^2\bound^2(1+\log(\lambda))},\frac{\delta}{2\omega\bound} \right\}}\right]\label{eq:dom_con}\\
%            &=0 \label{eq:conv_err}
%        \end{align}
%        \end{small}
%        Where \cref{eq:tower} comes from the tower property for conditional expectation. \cref{eq:bound_se} comes from \cref{sub-Gaussian:estimator} and \cref{def:SE}. \cref{eq:dom_con} comes from $\bound$ being a monotonically decreasing sequence implying that the term inside the expectation is dominated by $2e^{-\min\left\{\frac{\lambda \delta^2}{2\sigma^2M_0^2(1+\log(\lambda))},\frac{\delta}{2\omega M_0} \right\}}$, an integrable function. This domination by an integrable function allows us to use the dominated convergence theorem to switch the limit and the integral. \cref{eq:conv_err} then arises from \cref{thm:convergence-of-moments} and the definition of $\bound$.
%    \end{proof}
%
%  \subsection{Uncertainty Set and Stopping Criterion}\label{apdx:us_ci}
%  We present the proofs for the uncertainty set and stopping criterion from \cref{subsec:cons}.
%  \begin{corollary}[\cref{coll:credible-interval}]
%    An uncertainty set of level $1 - \alpha$ for $\rho_k^\lambda$
%    is 
%    \begin{equation} \label{eq:credible-interval-M1}
%    \tilde  \rho_k^\lambda \pm \epsilon,
%    \end{equation}
%    where,
%    \begin{small}
%    \begin{equation}
%        \epsilon = 
%        \begin{cases}
%            \sqrt{2 \log(2/\alpha)  \frac{\sigma^2 M^2_{k- \lambda}(1+\log(\lambda))}{\lambda}} & \text{if }\log(2 / \alpha) \leq \frac{\lambda \sigma^2 (1 + \log(\lambda))}{\omega^2}\\
%            \frac{2\log(2/\alpha)\omega\bound}{\lambda} & \text{if } \log(2 / \alpha) > \frac{\lambda \sigma^2 (1 + \log(\lambda))}{\omega^2}. 
%        \end{cases}
%    \end{equation}
%    \end{small} 
%\end{corollary}
%\begin{proof}
%    Using the sub-Exponential variance from \cref{sub-Gaussian:estimator}, the tail bound result from Proposition 2.9 of \cite{wainwright_2019},
%    \begin{small}
%    \begin{equation}
%      \mathbb{P}\left(\left| \tilde \rho_{k}^\lambda - \rho_{k}^\lambda \right| > \epsilon | \siga \right) \leq  2\exp\left(- \min\left(\frac{\lambda\epsilon^2}{2 \sigma^2 M^2_{k- \lambda} (1+ \log(\lambda))},\frac{\lambda \epsilon}{2 \omega \bound}\right)\right).
%    \end{equation}
%    \end{small}
%    From this tail probability it should be clear that the high probability region is controlled by the 
%    choice of $\epsilon$ thus if we choose $\epsilon$ such that it lines up with a specific quantile $\alpha$ 
%    we will have our desired confidence region.
%    \begin{small}
%    \begin{equation}
%        \alpha =  2\exp\left(- \min\left(\frac{\lambda\epsilon^2}{2 \sigma^2 M^2_{k- \lambda} (1+ \log(\lambda))},\frac{\lambda \epsilon}{2 \omega \bound}\right)\right). 
%    \end{equation}
%    \end{small}
%    Solving for $\epsilon$ and splitting the cases based on $\log(2/\alpha)$ supplies the desired result.
%\end{proof}
%
%We finish this section by describing the methodology by which to derive the error control condition for the stopping criterion. The process will 
%be the same for both types of errors; thus, we will show the work only for the first error type. 
%
%\begin{corollary}[\cref{corr:stopping}]
%    Given $\upsilon$, $\delta_I$, $\xi_I$, $\delta_{II}$, $\xi_{II}$ as defined in point \ref{stop-cond-desc} and a sampling matrix satisfying \cref{def:JL}, with $\delta_I$ and $\upsilon$ being chosen in such a way that then the two error types are controlled by
%    \begin{small}
%    \begin{equation} \label{eq:actual-typeI-control1}
%        \begin{aligned}
%        &\bound \leq \min\left\{\frac{\lambda \upsilon^2(1 - \delta_I)^2}{2\log(1/\xi_I)\sigma^2 \bound (1+ \log(\lambda))},\frac{\lambda\upsilon(1-\delta_I)}{2\log(1/\xi_I) \omega }\right\}\\
%        &\Rightarrow \mathbb{P}\left[ \tilde \rho_{k+1}^\lambda > \upsilon, \rho_k^\lambda \leq \delta_I\upsilon \bigg{\vert} \mathcal{F}_{k-\lambda+1} \right] < \xi_I,
%        \end{aligned}
%        \end{equation}
%    \end{small}
%        and
%    \begin{small}
%    \begin{equation} \label{eq:actual-typeII-control1}
%        \begin{aligned}
%        &\bound \leq \min\left\{\frac{\lambda \upsilon^2(\delta_{II}-1)^2}{2\log(1/\xi_{II})\sigma^2 \bound (1+ \log(\lambda))},\frac{\lambda\upsilon(\delta_{II} - 1)}{2\log(1/\xi_{II}) \omega }\right\}\\
%        &\Rightarrow \mathbb{P}\left[ \tilde \rho_{k+1}^\lambda \leq  \upsilon, \rho_k > \delta_{II} \upsilon \bigg{\vert} \mathcal{F}_{k-\lambda+1} \right] < \xi_{II}.
%        \end{aligned}
%        \end{equation}
%    \end{small}.
%\end{corollary}
%\begin{proof}
%First,
%\begin{small}
%\begin{align}
%&\mathbb{P}\left( \tilde \rho_k^\lambda > \upsilon, \rho_k^\lambda \leq \delta_I \upsilon \bigg{\vert} \mathcal{F}_{k-\lambda+1} \right) \notag \\
%&\leq \mathbb{P}\left( \tilde \rho_k^\lambda - \rho_k^\lambda> \upsilon(1 - \delta_I), \rho_k^\lambda \leq \delta_I \upsilon \bigg{\vert} \mathcal{F}_{k-\lambda+1} \right)  \\
%& \leq \mathbb{P}\left(\tilde  \rho_k^\lambda - \rho_k^\lambda> \upsilon(1 - \delta_I) \bigg{\vert} \mathcal{F}_{k-\lambda+1} \right)
%\end{align}
%\end{small}
%    Using the sub-Exponential variance from \cref{sub-Gaussian:estimator} and the tail bound result from Proposition 2.9 of \cite{wainwright_2019},
%    \begin{small}
%    \begin{align}
%        &\mathbb{P}\left(\tilde \rho_{k}^\lambda - \rho_k^\lambda > \upsilon (1-\delta_I) \right)  \notag \\
%        %& \quad \quad \leq  \exp\left(- \min\left(\frac{\lambda \upsilon^2 (1-\delta_I)^2}{2 \sigma^2 M_{k- \lambda + 1} (1+ \log(\lambda))},\frac{\lambda \upsilon (1 - \delta_I)}{2\omega \sqrt{M_k}}\right)\right)\\
%        & \quad \quad \leq  \exp\left(- \min\left(\frac{\lambda \upsilon^2 (1-\delta_I)^2}{2 \sigma^2 \bound^2 (1+ \log(\lambda))},\frac{\lambda \upsilon (1 - \delta_I)}{2\omega \bound}\right)\right),
%    \end{align}
%    \end{small} 
%     Thus, when $\bound$ satisfies \cref{eq:actual-typeI-control}, the right-hand side of the preceding inequality is bounded by $\xi_I$.
%We can repeat this argument to show that \cref{eq:actual-typeII-control} is true.
%\end{proof}
%
%  \section{Relative bound for $\tilde \iota_k^\lambda$} \label{apdx:rel_bound}
%  Here we define the relative error bound used at the end of the proof of \cref{lem:rel-of-iota}. We present the exact derivation of this bound in the following lemma.
%  
%  \begin{lemma}[\cref{lem:rel-of-iota}]
%    Under the conditions of \cref{thm:convergence-of-moments}, $\forall \delta > 0$  
%    \begin{small}
%    \begin{equation}
%    \begin{aligned}
%        &\pr \left(\left|\tilde \iota_k^\lambda - \frac{\sum_{i = k - \lambda +1}^k (\ex[\|\tilde r_i \|_2^2 | \mathcal{F}_{i-1}])^2}{\lambda}\right| > \delta \right)\\
%         &\leq (1+\lambda)\exp\left( - \frac{\delta^2 \lambda}{2\sigma^2\left(2 + \left(\frac{\delta^2 \lambda}{(1+ \log(\lambda))}\right)^{1/4}\right)^2 (1+\log(\lambda))}\right)
%    \end{aligned}       
%    \end{equation}
%    \end{small} 
%\end{lemma}
%
%\begin{proof}
%    Using the definition of $\tilde \iota_k^\lambda$ we have
%    \begin{small}
%    \begin{align}
%        &\pr\left(\left|\frac{\tilde \iota_k^\lambda - \frac{\sum_{i = k - \lambda +1}^k (\ex[\|\tilde r_i \|_2^2 | \mathcal{F}_{i-1}])^2}{\lambda}}{\bound^2}\right| > \delta\bigg| \siga\right)\\
%         &\quad \quad=\pr\left(\left|\sum_{i=k-\lambda + 1}^k\frac{ \|\tilde r_i\|_2^4 - (\ex[\|\tilde r_i \|_2^2 | \mathcal{F}_{i-1}])^2}{\lambda\bound^2} \right|> \delta \bigg| \siga\right)  \\
%        &\quad \quad \leq \pr\left(\sum_{i=k-\lambda + 1}^k \left|\frac{ \|\tilde r_i\|_2^4 - (\ex[\|\tilde r_i \|_2^2 | \mathcal{F}_{i-1}])^2}{\lambda\bound^2} \right|> \delta \bigg| \siga\right) \\
%        & \quad \quad  \leq \pr\left(\sum_{i=k-\lambda + 1}^k \left|\frac{ \|\tilde r_i\|_2^2 - \ex[\|\tilde r_i \|_2^2 | \mathcal{F}_{i-1}]}{\lambda\bound} \right| \left|\frac{ \|\tilde r_i\|_2^2 + \ex[\|\tilde r_i \|_2^2 | \mathcal{F}_{i-1}]}{\bound}\right|> \delta \bigg| \siga\right)\label{eq:whole1}.
%    \end{align}
%    \end{small}
%    Then by defining a variable, $G > 2$, to partition \cref{eq:whole1} into disjoint sets and using the definition of measure,
%    \begin{small}
%    \begin{align}
%        &\pr\left(\sum_{i=k-\lambda + 1}^k \left|\frac{ \|\tilde r_i\|_2^2 - \ex[\|\tilde r_i \|_2^2 | \mathcal{F}_{i-1}]}{\lambda\bound} \right| \left|\frac{ \|\tilde r_i\|_2^2 + \ex[\|\tilde r_i \|_2^2 | \mathcal{F}_{i-1}]}{\bound}\right|> \delta \bigg| \siga\right) \\  
%        &\quad \quad =\pr\bigg(\sum_{i=k-\lambda + 1}^k \left|\frac{ \|\tilde r_i\|_2^2 - \ex[\|\tilde r_i \|_2^2 | \mathcal{F}_{i-1}]}{\lambda\bound} \right| \left|\frac{ \|\tilde r_i\|_2^2 + \ex[\|\tilde r_i \|_2^2 | \mathcal{F}_{i-1}]}{\bound}\right|> \delta , \\ 
%         &\quad \quad \quad \quad\bigcap_{i=k-\lambda + 1}^k \left\{\left|\frac{ \|\tilde r_i\|_2^2 + \ex[\|\tilde r_i \|_2^2 | \mathcal{F}_{i-1}]}{\bound}\right|\leq G\right\} \bigg| \siga\bigg)  \notag\\
%         & \quad \quad+\pr\bigg(\sum_{i=k-\lambda + 1}^k \left|\frac{ \|\tilde r_i\|_2^2 - \ex[\|\tilde r_i \|_2^2 | \mathcal{F}_{i-1}]}{\lambda\bound} \right| \left|\frac{ \|\tilde r_i\|_2^2 + \ex[\|\tilde r_i \|_2^2 | \mathcal{F}_{i-1}]}{\bound}\right|> \delta , \notag\\ 
%         &\quad \quad \quad \quad\bigcup_{i=k-\lambda + 1}^k \left\{\left|\frac{ \|\tilde r_i\|_2^2 + \ex[\|\tilde r_i \|_2^2 | \mathcal{F}_{i-1}]}{\bound}\right|> G\right\} \bigg| \siga\bigg)\notag\\
%         & \label{int-bound1} \leq\pr\bigg(\sum_{i=k-\lambda + 1}^k \left|\frac{ \|\tilde r_i\|_2^2 - \ex[\|\tilde r_i \|_2^2 | \mathcal{F}_{i-1}]}{\lambda\bound} \right| > \frac{\delta}{G} \bigg| \siga \bigg)\\ &\quad \quad \quad + \pr\bigg(\bigcup_{i=k-\lambda + 1}^k \left\{\left|\frac{ \|\tilde r_i\|_2^2 + \ex[\|\tilde r_i \|_2^2 | \mathcal{F}_{i-1}]}{\bound}\right|> G\right\} \bigg| \siga\bigg)\notag.
%    \end{align}
%    \end{small}
%    From here we will present the bounds for the left and right terms of \cref{int-bound1} separately. For the left term of \cref{int-bound1} we use \cref{eq:chernoff} and have
%    \begin{small}
%    \begin{align}
%        \label{rchernoff1}\pr\bigg(\sum_{i=k-\lambda + 1}^k \left|\frac{ \|\tilde r_i\|_2^2 - \ex[\|\tilde r_i \|_2^2 | \mathcal{F}_{i-1}]}{\lambda \bound} \right| > \frac{\delta}{G}\bigg| \siga\bigg)\leq & \exp \left(\frac{t^2 \sigma^2 (1+ \log(\lambda))}{2\lambda} - \frac{\delta t}{G}\right)\\
%        &\label{rmint1}\leq \exp\left( - \frac{\delta^2 \lambda}{2G^2 \sigma^2(1+\log(\lambda))}\right), 
%    \end{align}
%    \end{small}
%    where \cref{rmint1} comes from minimizing \cref{rchernoff1} in terms of $t$. We next address the right side of \cref{int-bound1} for which we have
%    \begin{small}
%    \begin{align}
%        &\pr\bigg(\bigcup_{i=k-\lambda + 1}^k \left\{\left|\frac{ \|\tilde r_i\|_2^2 + \ex[\|\tilde r_i \|_2^2 | \mathcal{F}_{i-1}]}{\bound}\right|> G\right\} \bigg| \siga\bigg)  \\
%         &\quad \quad  =\pr\bigg(\bigcup_{i=k-\lambda + 1}^k \left\{\left|\frac{ \|\tilde r_i\|_2^2 - \ex[\|\tilde r_i \|_2^2 | \mathcal{F}_{i-1}] + 2 \ex[\|\tilde r_i \|_2^2 | \mathcal{F}_{i-1}]}{\bound}\right|> G \right\}\bigg| \siga\bigg)\\
%        &\label{bounddef1}\quad \quad \leq \pr\bigg(\bigcup_{i=k-\lambda + 1}^k \left\{\left|\frac{ \|\tilde r_i\|_2^2 - \ex[\|\tilde r_i \|_2^2 | \mathcal{F}_{i-1}]}{\bound}\right| + 2> G\right\} \bigg| \siga\bigg)  \\
%        %&\quad \quad =\pr\bigg(\bigcup_{i=k-\lambda + 1}^k \left\{\left| \|\tilde r_i\|_2^2 - \ex[\|\tilde r_i \|_2^2 | \mathcal{F}_{i-1}] \right|> G - 2\bound^2 \right\}\bigg| \siga\bigg)\\
%        & \quad \quad \leq \sum_{i=k-\lambda + 1}^k\pr\bigg(\left|\frac{ \|\tilde r_i\|_2^2 - \ex[\|\tilde r_i \|_2^2 | \mathcal{F}_{i-1}]}{\bound}\right|> G - 2 \bigg| \siga\bigg)\\
%        &\label{lchernoff1} \quad \quad \leq \lambda \exp \left(\frac{t^2\sigma^2 }{2} - t\left(G - 2\right)\right)\\
%        & \label{mincher1} \quad \quad \leq \lambda \exp\left( -\frac{\left(G - 2\right)^2}{2\sigma^2} \right),
%    \end{align}
%\end{small}
%    where \cref{bounddef1} comes from \cref{rtoM},
%    \cref{lchernoff1} comes from the \cref{eq:chernoff}, and \cref{mincher1} comes from minimizing \cref{lchernoff1} in terms of $t$. Putting both parts together gives us,
%    \begin{small}
%    \begin{align}
%        &\pr\left(\left|\frac{\tilde \iota_k^\lambda - \iota_k^\lambda}{\bound^2}\right| > \delta\bigg| \siga\right) \\
%        &\quad \quad\leq \inf_{G > 2} \exp\left( - \frac{\delta^2 \lambda}{2G^2 \sigma^2(1+\log(\lambda))}\right) + \lambda \exp\left( -\frac{\left(G - 2\right)^2}{2\sigma^2} \right). \label{final-rate-iota1}
%    \end{align}       
%    \end{small}
%    We can then observe that when $G \geq 2 + \left(\frac{\delta^2 \lambda}{(1+ \log(\lambda))}\right)^{1/4} $ it is the case that
%    \begin{equation}
%        \exp\left( - \frac{\delta^2 \lambda}{2G^2\sigma^2 (1+\log(\lambda))}\right) \geq \exp\left( -\frac{\left(G - 2\right)^2}{2\sigma^2} \right). 
%    \end{equation}
%    Thus, if we let $Y = 2 + \left(\frac{\delta^2 \lambda}{(1+ \log(\lambda))}\right)^{1/4}$ we can upper bound the right-hand side of \cref{final-rate-iota1} in the following manner,
%    \begin{small}
%    \begin{align}
%        &\inf_{G > 2} \exp\left( - \frac{\delta^2 \lambda}{2G^2 \sigma^2 (1+\log(\lambda))}\right) +\lambda \exp\left( -\frac{\left(G - 2\bound^2\right)^2}{2\sigma^2} \right)\\
%        &\leq \inf_{G > Y} (1+\lambda)\exp\left( - \frac{\delta^2 \lambda}{2G^2\sigma^2  (1+\log(\lambda))}\right)\\%\label{secondary-iota-bound}\\
%        &\leq (1+\lambda)\exp\left( - \frac{\delta^2 \lambda}{2\sigma^2\left(2 + \left(\frac{\delta^2 \lambda}{(1+ \log(\lambda))}\right)^{1/4}\right)^2 (1+\log(\lambda))}\right).
%    \end{align}
%    \end{small}
%\end{proof}
%
%
%\section{Distribution Constants for Johnson - Lindenstrauss Sampling methods}
%In the differential privacy case, to be able to use common sampling methods for our estimators,
%we must compute the constants in the Johnson-Lindenstrauss property (see \cref{def:JL}). We first present the constants in the following table then present how the constants were derived. 
%
%\begin{table}
%    \centering
%    \caption{Values of $C$ and $\omega$ in \cref{def:JL} for common sampling methods.}
%    \label{table-JL-constant-values}
%    \begin{tabular}{lccccc}
%          \toprule
%           &$C$ & $\omega$\\
%           \midrule
%          Gaussian Matrix \cite{Dasgupta2003AnEP}  & 0.23467 & .1127\\
%           Achlioptas \cite{ACHLIOPTAS2003671}  & 0.23467 & .1127\\
%           FJLT \cite{Ailon2009TheFJ} & 0.03125 & .0625\\ 
%           \bottomrule
%       \end{tabular} 
%\end{table}
%
%We will first find the constants for Achlioptas sketching and Gaussian sketching \cite{ACHLIOPTAS2003671}.
%
%\begin{corollary}
%    The variance constant for the Gaussian and Achlioptas sampling methods will be  
%    \begin{equation}
%    C = 0.23467.
%    \end{equation}
%  \end{corollary} 
%  \begin{proof}
%    Noting from \cite{ACHLIOPTAS2003671} that for a unit vector x $\mathbb{P}(\|Sx\|_2^2 > (1-\delta)p/m) \geq \mathbb{P}(\|S'x\|_2^2 > (1+\delta)p/m)$
%    it is necessary to only bound the tail probability of $\mathbb{P}(\|S'x\|_2^2 > (1-\delta)p/m)$. To do this we will 
%    find a constant $C$ such that $\mathbb{P}(\|S'x\|_2^2 > (1-\delta)p/m) \leq \exp\left(\frac{-\delta^2}{2C}\right)$.
%    Using equation (16) from \cite{ACHLIOPTAS2003671} we will have that 
%    \begin{equation}
%        \mathbb{P}(\|S'x\|_2^2 > (1-\delta)p/m) \leq \left(1+\frac{\delta}{2(1+\delta)}+\frac{3\delta^2}{8(1+\delta)^2}\right)^k \exp\left(\frac{k\delta(1-\delta)}{2(1+\delta)}\right).
%    \end{equation}
%    Thus, we will try to find the $C$ such that 
%    \begin{equation}\label{achlio_start}
%        \left(1+\frac{\delta}{2(1+\delta)}+\frac{3\delta^2}{8(1+\delta)^2}\right)^p \exp\left(\frac{p\delta(1-\delta)}{2(1+\delta)}\right) \leq \exp\left(-Cp\delta^2\right). 
%    \end{equation}
%    Taking the $\log$ of both sides of \cref{achlio_start} we have
%    \begin{equation}
%        p\log\left(1-\frac{\delta}{2(1+\delta)}+\frac{3\delta^2}{8(1+\delta)^2}\right) + \frac{p\delta(1-\delta)}{2(1+\delta)} \leq -Cp\delta^2.
%    \end{equation}
%    Which implies that 
%    \begin{equation}
%        -\log\left(1-\frac{\delta}{2(1+\delta)}+\frac{3\delta^2}{8(1+\delta)^2}\right) - \frac{\delta(1-\delta)}{(1+\delta)} \geq C \delta^2.
%    \end{equation}
%    Which after rearranging will give us that 
%    \begin{equation}\label{achlio_max}
%        C \leq \frac{-2 p\log\left(1-\frac{\delta}{2(1+\delta)}+\frac{3\delta^2}{8(1+\delta)^2}\right)- \frac{p\delta(1-\delta)}{(1+\delta)}}{-\delta^2}.
%    \end{equation}
%    Finding a positive local min of the equation on the right-hand side of \cref{achlio_max} gives us that 
%    \begin{equation}
%        C \leq 0.235467.
%    \end{equation}
%  \end{proof}
%  To examine the FJLT case it is necessary to compute the constants from the 
%  proof in \cite{Ailon2009TheFJ}. Noting of course that the method 
%  proposed in \cite{Ailon2009TheFJ} is not exactly the same as the FJLT, it is based on 
%  the same idea and should provide a good enough constant for demonstrative purposes.
%  In order to determine the constants it is necessary to apply \cite[Lemma 2.3]{Ailon2009TheFJ}.
%  \begin{lemma}[Lemma 2.3 Ailon et al.]\label{Ailon:key}
%    With probability at least $1-1/20n$
%    \begin{itemize}
%      \item $q/2 \leq Z_i \leq 2q$ for all $i = 1,\dots,d$ and 
%      \item $dq(1-\delta) \leq \sum_{i=1}^d Z_i \leq dq(1+\delta)$
%    \end{itemize}
%  \end{lemma}
%  It should be noted that q is the probability a row is selected. Z is the sum of the squared elements 
%  of the projection residual that are selected by the row sampling.
%  \begin{corollary}
%    The variance constant for the FJLT will be 
%    \begin{equation}
%    C = \frac{1}{32}
%    \end{equation}
%  \end{corollary}
%  \begin{proof}
%    To get the values to determine the variance it is going to be necessary to first complete the proof of the L2 case 
%    from \cite{Ailon2009TheFJ}. In order to get the constants on the probability bound. In their proof, it is assumed w.l.o.g 
%    that $\|r_k\|_2^2 = 1$. From their proof we then have 
%    \begin{equation}\label{bound:ailon}
%      \mathbb{P}\left[\|S_{k+1} r_k\|_2^2 > (1+\delta) \sum_{i=1}^p Z_i/q\right] \leq \exp\left(-\delta \lambda \sum_{i=1}^d Z_i/q + \xi \lambda^2 \sum_{i=1}^p (Z_i/q)^2\right).
%    \end{equation}
%    Setting  $\lambda = \frac{\delta \sum_{i=1}^p Z_i/q}{2\xi\sum_{i=1}^p (Z_i/q)^2}$ and plugging it  into \cref{bound:ailon} results in 
%    \begin{align}
%      \mathbb{P}\left[\sum_{i=1}^p y_i^2 > (1+\delta) \sum_{i=1}^d Z_i/q\right] &\leq \exp\left(- \frac{\delta^2 (\sum_{i=1}^d Z_i/q)^2}{4\xi\sum_{i=1}^d (Z_i/q)^2}\right)\label{eq:ailon:2}\\
%      \cref{eq:ailon:2} \leq \exp\left(- \frac{p \delta^2}{64 \xi}\right),\label{delt_small}
%    \end{align}
%    Where \cref{delt_small} comes from $\delta$ being small enough to avoid convergence issues and using \cref{Ailon:key}. 
%    Noting the same size tail estimate can be derived for the left tail we have 
%    \begin{equation}
%      \mathbb{P}\left[\sum_{i=1}^p y_i^2 > (1+\delta) k \right] \leq  2 \exp\left(- \frac{p\delta^2}{64 \xi}\right).
%    \end{equation}
%    Taking $\xi = 1$ to ensure convergence, this is exactly the sub-Gaussian part of sub-Exponential tail giving us that 
%    \begin{equation}
%        C = \frac{1}{32}.
%    \end{equation}
%  \end{proof}
